# Supplementary material for: Implicit Geometry and Interaction Embeddings Improve Few-Shot Molecular Property Prediction
Source: arXiv:2302.02055 source file (2023-10-06)
Supplement: Supplementary file 1 [file main_supplementary.tex]

\documentclass{article}

\usepackage{microtype}
\usepackage{graphicx}
\usepackage{epstopdf}
\usepackage{subfigure}
\usepackage{booktabs} % for professional tables

\usepackage{amsmath}
\usepackage{multirow}
\usepackage[dvipsnames]{xcolor}
\usepackage{amsthm}   
\usepackage{amssymb}
\usepackage{wasysym}
\usepackage{bbm}
\usepackage{tikz}
\usetikzlibrary{calc}
\usetikzlibrary{arrows.meta}

\usepackage{hyperref}

\input{macro.tex}
\input{math_commands.tex}
\graphicspath{{figures/}}

\usepackage{icml2023}

\icmltitlerunning{Simplifying Graph Convolutional Networks (Supplementary Material)}

\begin{document}

\twocolumn[   %or twocolumn

\icmltitle{Simplifying Graph Convolutional Networks \\ (Supplementary Material)}

\icmlsetsymbol{equal}{*}

\begin{icmlauthorlist}
\icmlauthor{Aeiau Zzzz}{equal,to}
\icmlauthor{Bauiu C.~Yyyy}{equal,to,goo}
\icmlauthor{Cieua Vvvvv}{goo}
\icmlauthor{Iaesut Saoeu}{ed}
\icmlauthor{Fiuea Rrrr}{to}
\icmlauthor{Tateu H.~Yasehe}{ed,to,goo}
\icmlauthor{Aaoeu Iasoh}{goo}
\icmlauthor{Buiui Eueu}{ed}
\icmlauthor{Aeuia Zzzz}{ed}
\icmlauthor{Bieea C.~Yyyy}{to,goo}
\icmlauthor{Teoau Xxxx}{ed}
\icmlauthor{Eee Pppp}{ed}
\end{icmlauthorlist}

\icmlaffiliation{to}{Department of Computation, University of Torontoland, Torontoland, Canada}
\icmlaffiliation{goo}{Googol ShallowMind, New London, Michigan, USA}
\icmlaffiliation{ed}{School of Computation, University of Edenborrow, Edenborrow, United Kingdom}

\icmlcorrespondingauthor{Cieua Vvvvv}{c.vvvvv@googol.com}
\icmlcorrespondingauthor{Eee Pppp}{ep@eden.co.uk}

\icmlkeywords{Machine Learning, ICML}
\vskip 0.3in

]

\appendix

\input{sections/supplementary.tex}
\clearpage

\bibliography{references}
\bibliographystyle{icml2023}
\end{document}
